# Supplementary material for: A Declarative System for Optimizing AI Workloads
Source: arXiv:2405.14696 source file (2024-05-29)
Supplement: Supplementary file 1 [file additionalworkloads.tex]

\subsection{Additional Workloads}
% \matt{While SAPPs are an exciting new class of AI workloads which \system{} is designed to support, it also helps users optimize more ``traditional" systems such as ones using Retrieval Augmented Generation (RAG).}
Beyond SAPPs, there are a number of workloads which \system{} is well-suited to implement given its relational model and optimizer.

\noindent {\bf Document-driven discovery.} Organizations and individuals often wish to extract insights from sets of documents. For example, investors may wish to examine the footnotes of public US banks' SEC filings to see if they are at risk of a liquidation event. As another example, database researchers may try to process five years of VLDB and SIGMOD papers to extract specific metadata of interest (e.g., how the number of figures in accepted papers has varied over time).
\mjf{why isn't this a SAPP?  Seems to meet all the criteria}

Such tasks can easily be performed using \system{}. As shown previously in \autoref{fig:email} and \autoref{fig:examples}, users simply provide their source documents as an input {\tt Dataset} and define the metadata they wish to extract using their own {\tt Schema}. They may also perform additional post-processing on the extracted metadata following the schema conversion.

\noindent {\bf Multimodal integration.} Users often wish to integrate multiple datasources of differing modalities in order to enhance their ability to extract quantitative insights. For example, an insurance company may collect photos of a car crash along with police reports to help determine whether the driver they insure is at fault or not. Similarly, firefighters may collect streaming video data along with live weather maps to try to pinpoint the location of a brush fire. Once again, \system{} can assist users with creating AI systems for such workloads by allowing users to write simple {\tt Schemas} against each data modality to extract quantitative fields of interest.

\noindent {\bf Schema matching.}
To manage large collections of structured data from different sources often requires matching schemata across different tables.
For example, a medical researcher may wish to perform a large-scale study that requires integrating new patient data collected by previous field studies together with new experimental observations.
Or, environmental scientists may want to analyze climate change using historical data collected with different sensors across different geographical regions.
With the use of \system{}, users can write a simple specification of the target {\tt Schema} using natural language, and let \system{} automatically infer how to extract and match the existing attributes from all source datasets.

\noindent {\bf RAG systems.} The Retrieval Augmented Generation (RAG) architecture has rapidly become a first-class use case for neural models in enterprise settings. They are characterized by a two-stage process: first, a retrieval model is used to identify a set of candidate input documents, and then a generation model is used to produce a high-quality output based on the inputs. Even this dead-simple architecture exhibits performance, cost, and quality tradeoffs when the system designer decides how many documents to fetch from a vector database in Step 1. Too few means the LLM may not have relevant information it needs, while too many means the system performs unnecessary queries. \matt{\system{} is designed to optimize for these types of tradeoffs, thus supporting RAG applications is quite natural.}

\tim{I find it confusing that you mention RAG here. Everything else are use cases, RAG is a technique to achieve a particular goal, e.g., schema matching. For me it is on the same level as model selection, code generation, etc,. which are all tools/techniques to achieve a specific goal.} 
\mjf{I also think the above examples except for RAG could be considered SAPPs - no?  If so, then it is indeed interesting that the system (or at least the insights underlying it) could be used to support RAG, which as Tim says, seems different from the others.}

\system\ is designed to use the RAG architecture in two different ways. First, it can employ RAG-style methods as part of its query plan. For example, consider \st{a topic summarization program in \autoref{fig:extraction-example}} the use case of topic summarization over a set of documents. If the input document is larger than any available model's maximum token size, \system\ can decide, during synthesis of the convert operation, to use a RAG-style method to make the subtask manageable. That is, it may: (1) decompose the input text into smaller chunks, (2) choose chunks that are both relevant and will fit in the model's context size, then (3) generate the output summary using the selected chunks. This is a purely "internal" RAG approach, which is invisible to the user.

\matt{Matt: Re-reading the paragraph above made me realize that it pretty much summarizes Chunwei's input token reduction technique, because I doubt 95\% of users have documents which cannot fit in the context of the newest models. The more I think about it, the more I understand Tim's comment that, at least in our worldview, RAG is a token-reduction optimization which has quality and runtime tradeoffs as well. The key point we want to make is that PZ can optimize your RAG system for you --- but I think that falls outside of ``workloads" and maybe this text should go into ``optimizations"? Perhaps we should reframe this subsection as illustrating how ``traditional workloads" can be represented as SAPPs. I.e. ``document-driven discovery is a SAPP where the input is ... multimodal integration is a SAPP which focuses on the extraction of structured fields from ... Schema matching is a SAPP in which ..." }

The system can also support "external" RAG applications in which the user has an external data store of documents. \system\ allows users to define their own datasources, and can use these sources as part of the query plan. We understand from talking with industrial contacts that one of the primary engineering challenges encountered when building RAG systems is managing the inevitable quality/runtime tradeoffs. For example, how many 
documents should be returned by the vector database in response to a query? Too many, and the system is unnecessarily slow; too few, and the system yields bad results. This kind of tradeoff is exactly what \system\ was designed to handle: we are currently working on an extension that will allow \system\ to optimize these external RAG database queries.

% \noindent {\bf Database Administration}

% Older content:

% \noindent {\bf }

% Functionalities we wish to highlight:
% \begin{itemize}
%     \item \textbf{Queries over text / PDFs}
%     \begin{itemize}
%         \item Searching Enron emails for ref. to Special Purpose Entities (SPEs) (i.e. fraud)
%         \item Matching investment hypothesis to companies' public filings
%     \end{itemize}
%     \item \textbf{Queries over images}
%     \begin{itemize}
%         \item Semantic search over image repos (``find a photo of my dog playing in the snow")
%         \item Satellite image classification (Amazon deforestation)
%         \item Stream classifiers (e.g. imagine having an Amber Alert which only requires updating the Alert prompt rather than re-training an image classifier)
%     \end{itemize}
%     \item \textbf{Multi-modal queries}
%     \begin{itemize}
%         \item Fake Amazon products \& reviews
%         \item Search over video / audio + transcription
%         \item Investment hypothesis (PDF + stock time-series data)
%     \end{itemize}
%     \item \textbf{Queries which require using RAG}
%     \begin{itemize}
%         \item Understanding my tax liability (querying IRS docs + tax law)
%         \item (Possibly investment hypothesis example; we may need to pre-process PDFs and perform RAG over their contents)
%     \end{itemize}
% \end{itemize}
